# Supplementary material for: Hardware Impairments Aware Transceiver Design for Full-Duplex Amplify-and-Forward MIMO Relaying
Source: arXiv:1703.10209 source file (2017-08-15)
Supplement: Supplementary file 1 [file main_Appendix.tex]

{\it{Proof to Lemma 2}:} Since $b_{k,1},b_{k,2} \in \real^{+}$, the real-valued nature of $r_{k,1},r_{k,2}$ can be directly concluded from (21). On the other hand, the value of $\tilde{\rm SENR}_k$ approaches to zero as $\tilde{a}_k \rightarrow 0$ and $\tilde{a}_k \rightarrow  \tilde{a}_k^{\infty}$, for nonzero values of noise and distortion components. Since the value of $\tilde{\rm SENR}_k$ remains positive, continues and differentiable in the range $\left(0,  \tilde{a}_k^{\infty} \right)$ there exists at least one maximum in this region. In this regard, two scenarios are probable. If $0<b_{k,1} < b_{k,2}$, then $r_{k,2}<0$ and $r_{k,1}$ is the only extrema in the positive region. On the other hand, if $b_{k,1} > b_{k,2} >0$ we have $r_{k,1},r_{k,2} \in  \real^{+}$. In this case we have   
{\small{\begin{align}
r_{k,1} = \frac{1}{b_{k,1} -b_{k,2}} + \frac{\sqrt{{b_{k,2}}/{b_{k,1}}}}{\left| b_{k,2}-b_{k,1} \right|} > \frac{1}{b_{k,1} -b_{k,2}} > \frac{1}{b_{k,1}}= \tilde{a}_k^{\infty}. \nonumber
\end{align}}}
The above argument concludes that we never face with two stationary points in the region $\left(0,  \tilde{a}_k^{\infty} \right)$, and the only root which is located in the aforementioned region, is the single SENR-maximizing point we have been looking for, i.e., $r_k^{\star}$. 

\begin{figure}[!t] \vspace{-0mm}
    \begin{center}
        \includegraphics[angle=0,width=0.99\columnwidth]{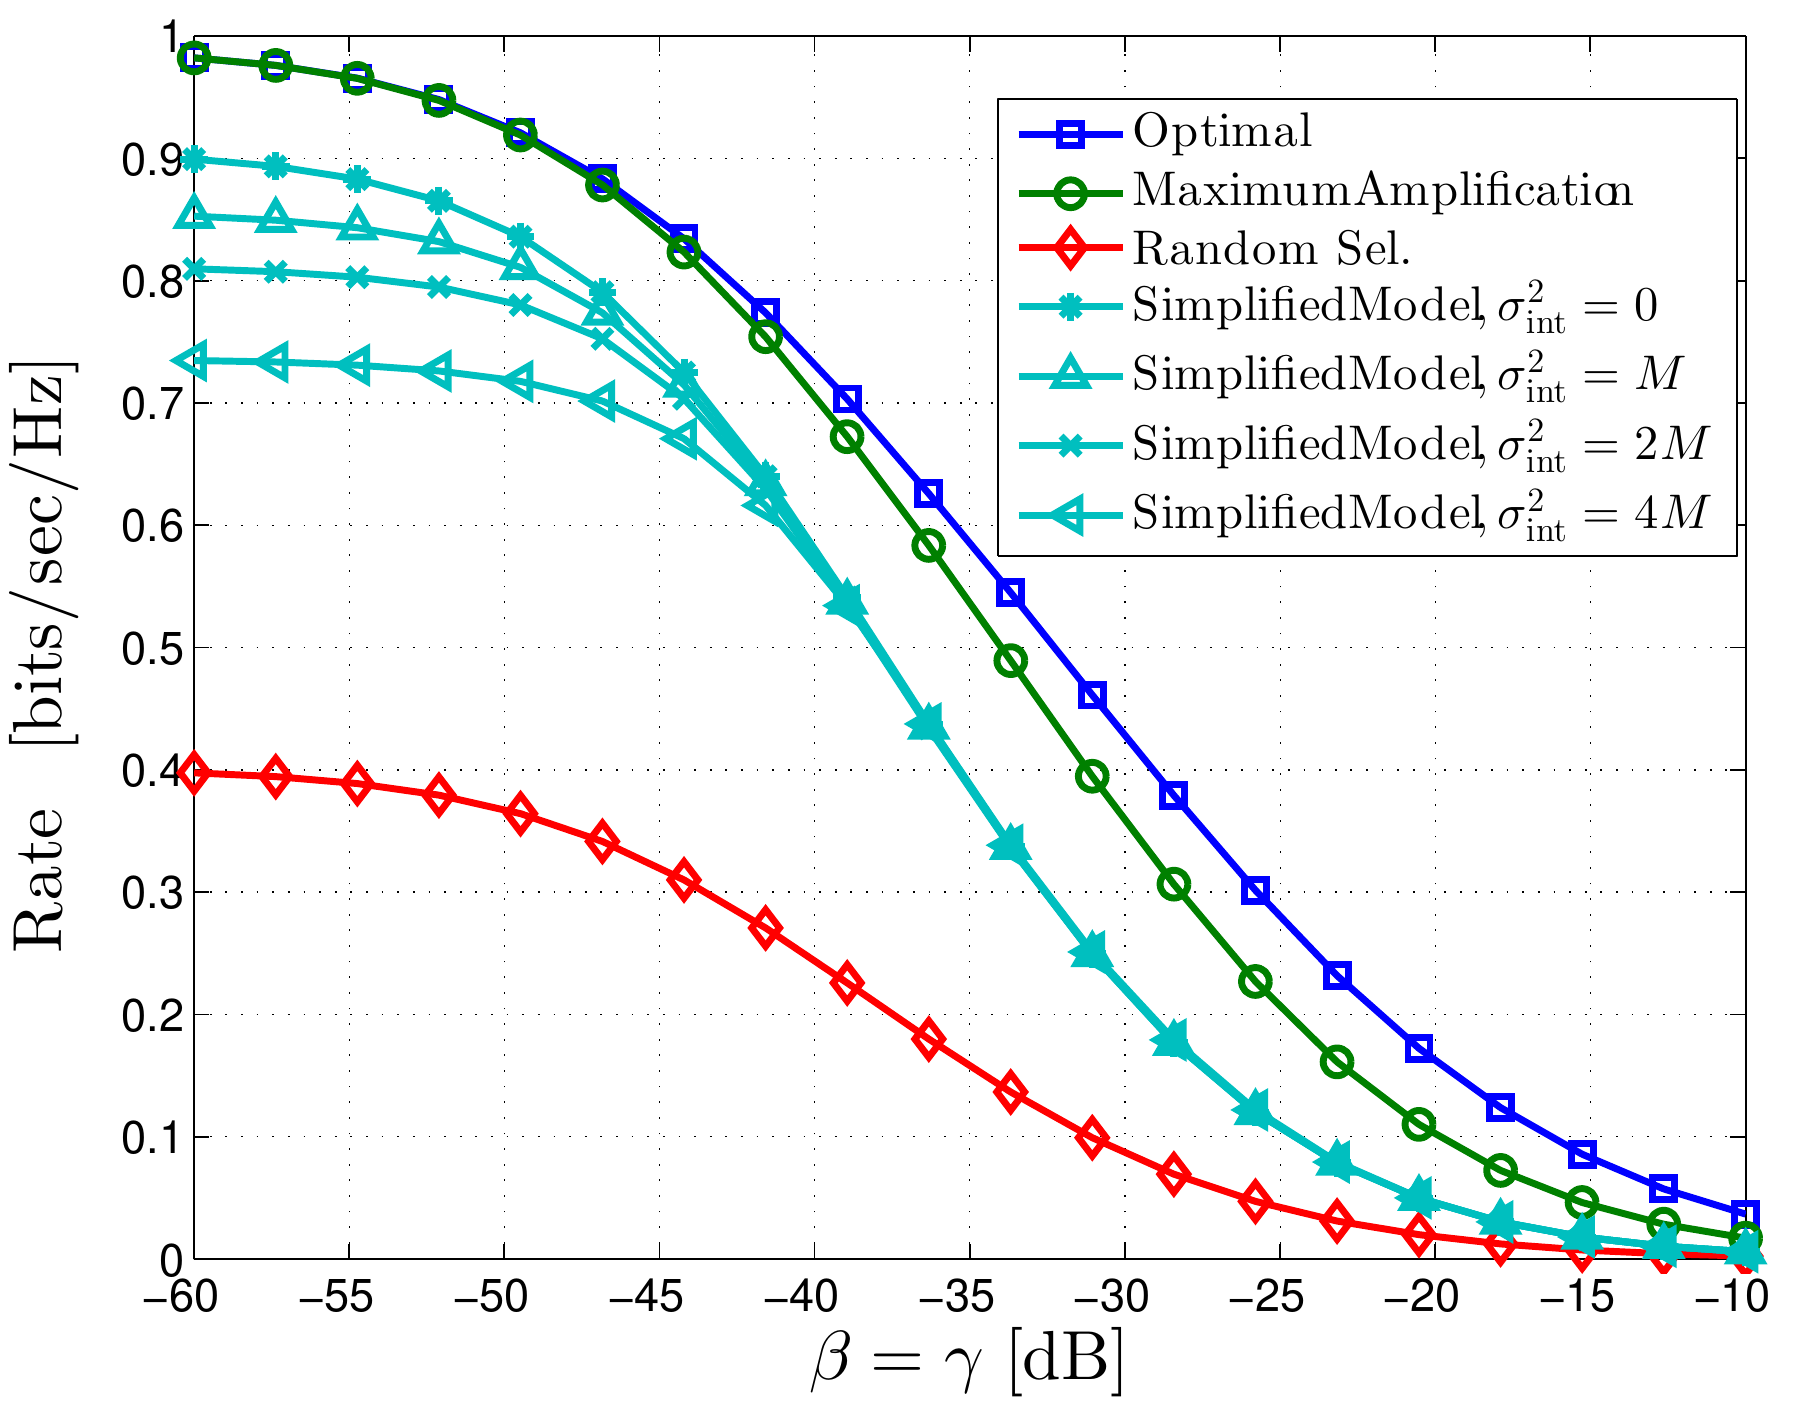}
				        %\fbox{model_rect6.pdf}
    \end{center} \vspace{-1mm}
    \caption{\small{Achievable rate [bits/sec/Hz] for the weakest end-to-end link vs. distortion coefficients $\eta,\beta$ [dB]. The gain is observed specially for low dynamic range region. }}
		\vspace{-0mm}
%\end{figure} 		
%\begin{figure}[!h] \vspace{-0mm}
      \begin{center}
      \includegraphics[angle=0,width=0.99\columnwidth]{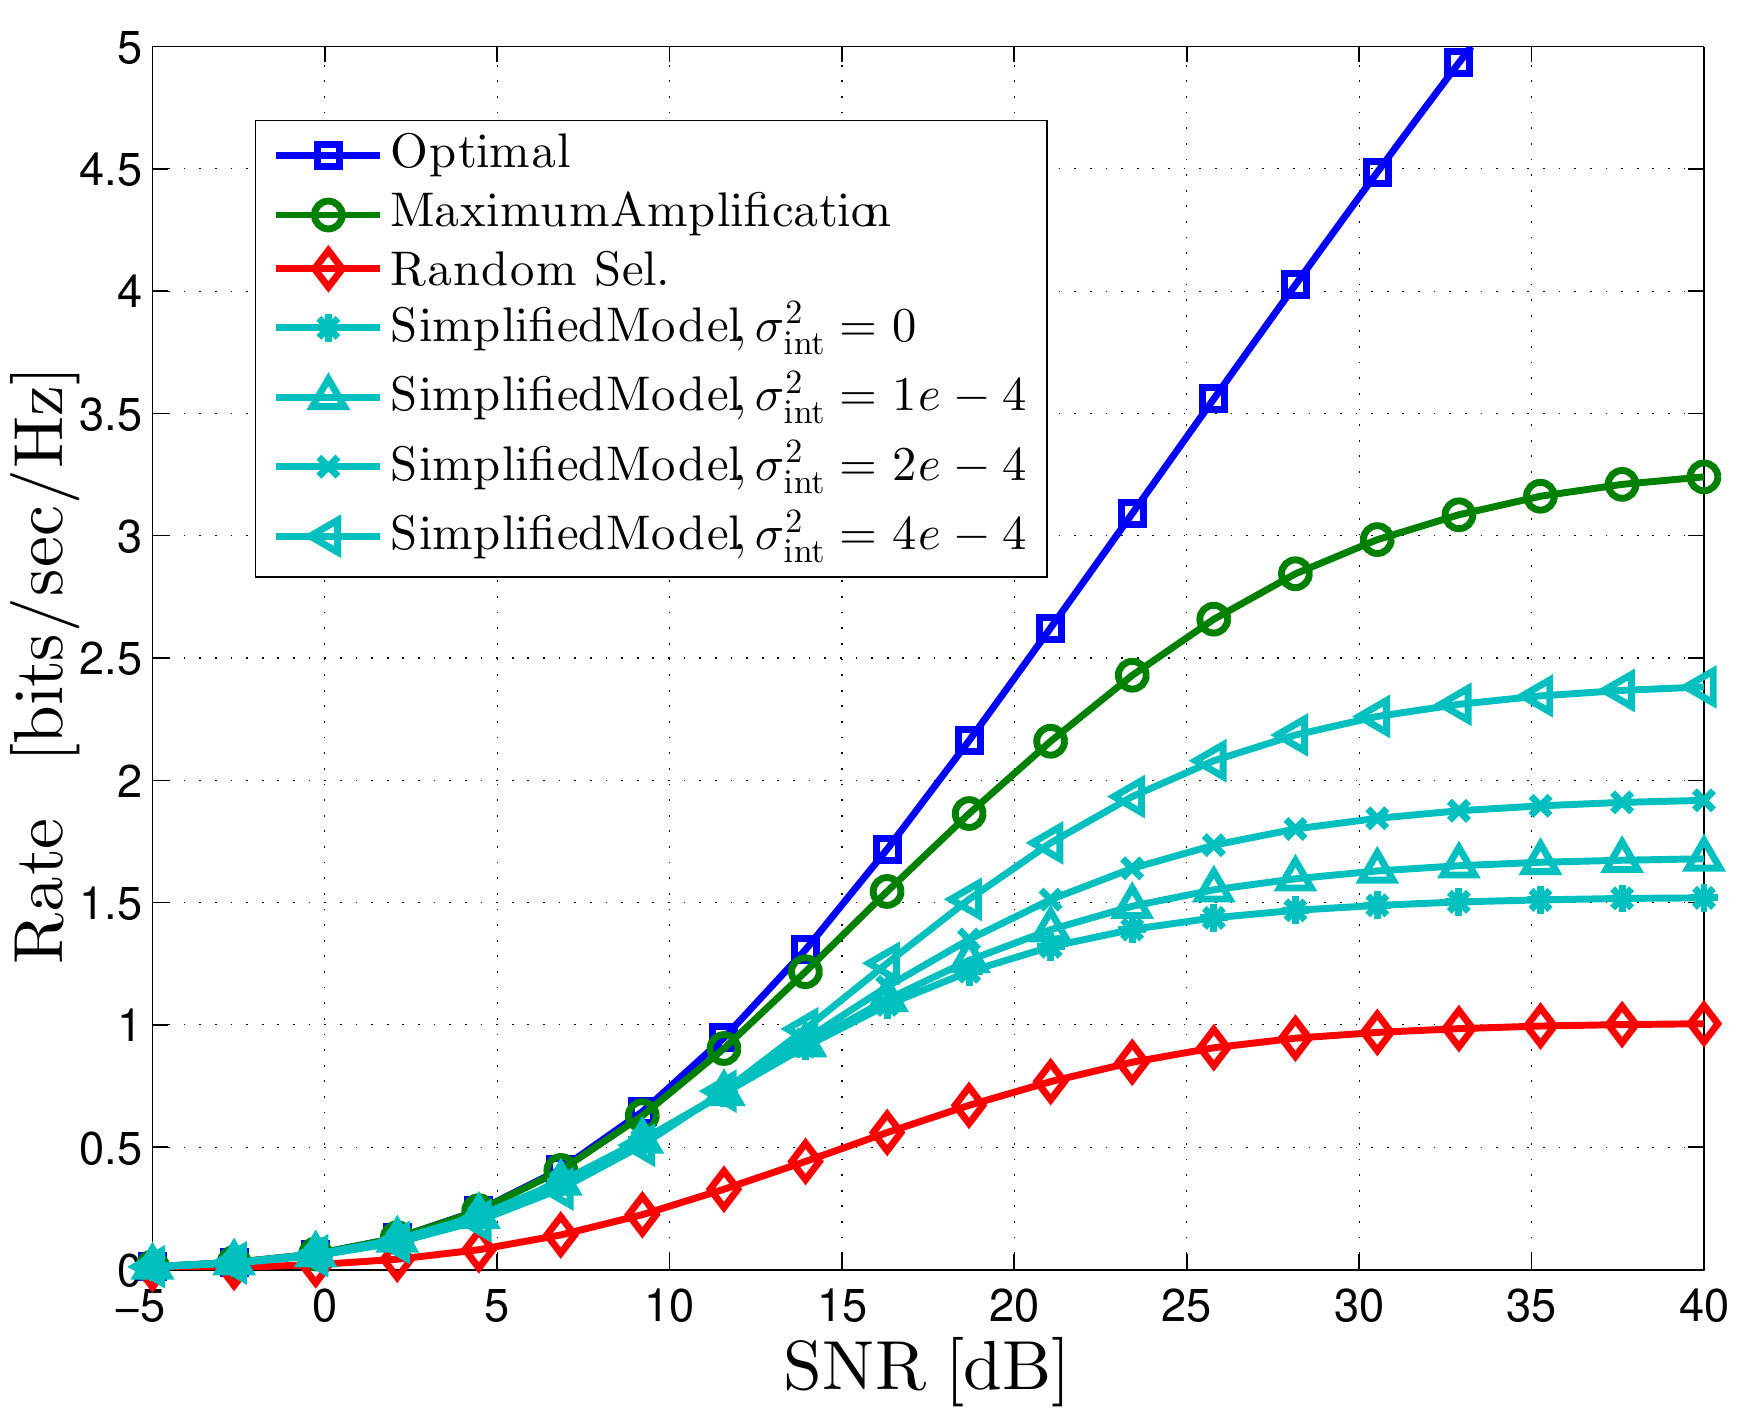}
				        %\fbox{model_rect6.pdf}
    \end{center} \vspace{-1mm}
    \caption{\small{Achievable rate [bits/sec/Hz] for the weakest end-to-end link vs. SNR [dB]. The significant gain is observed for the optimal design in high SNR region. ${\rm SNR} := \frac{P_s \mathcal{E}\{|{h}_{{\rm sr},k}|^2\}}{M}$. }}
		\vspace{-0mm}
\end{figure}

\begin{figure}[!t] \vspace{-0mm}
    \begin{center}
        \includegraphics[angle=0,width=0.99\columnwidth]{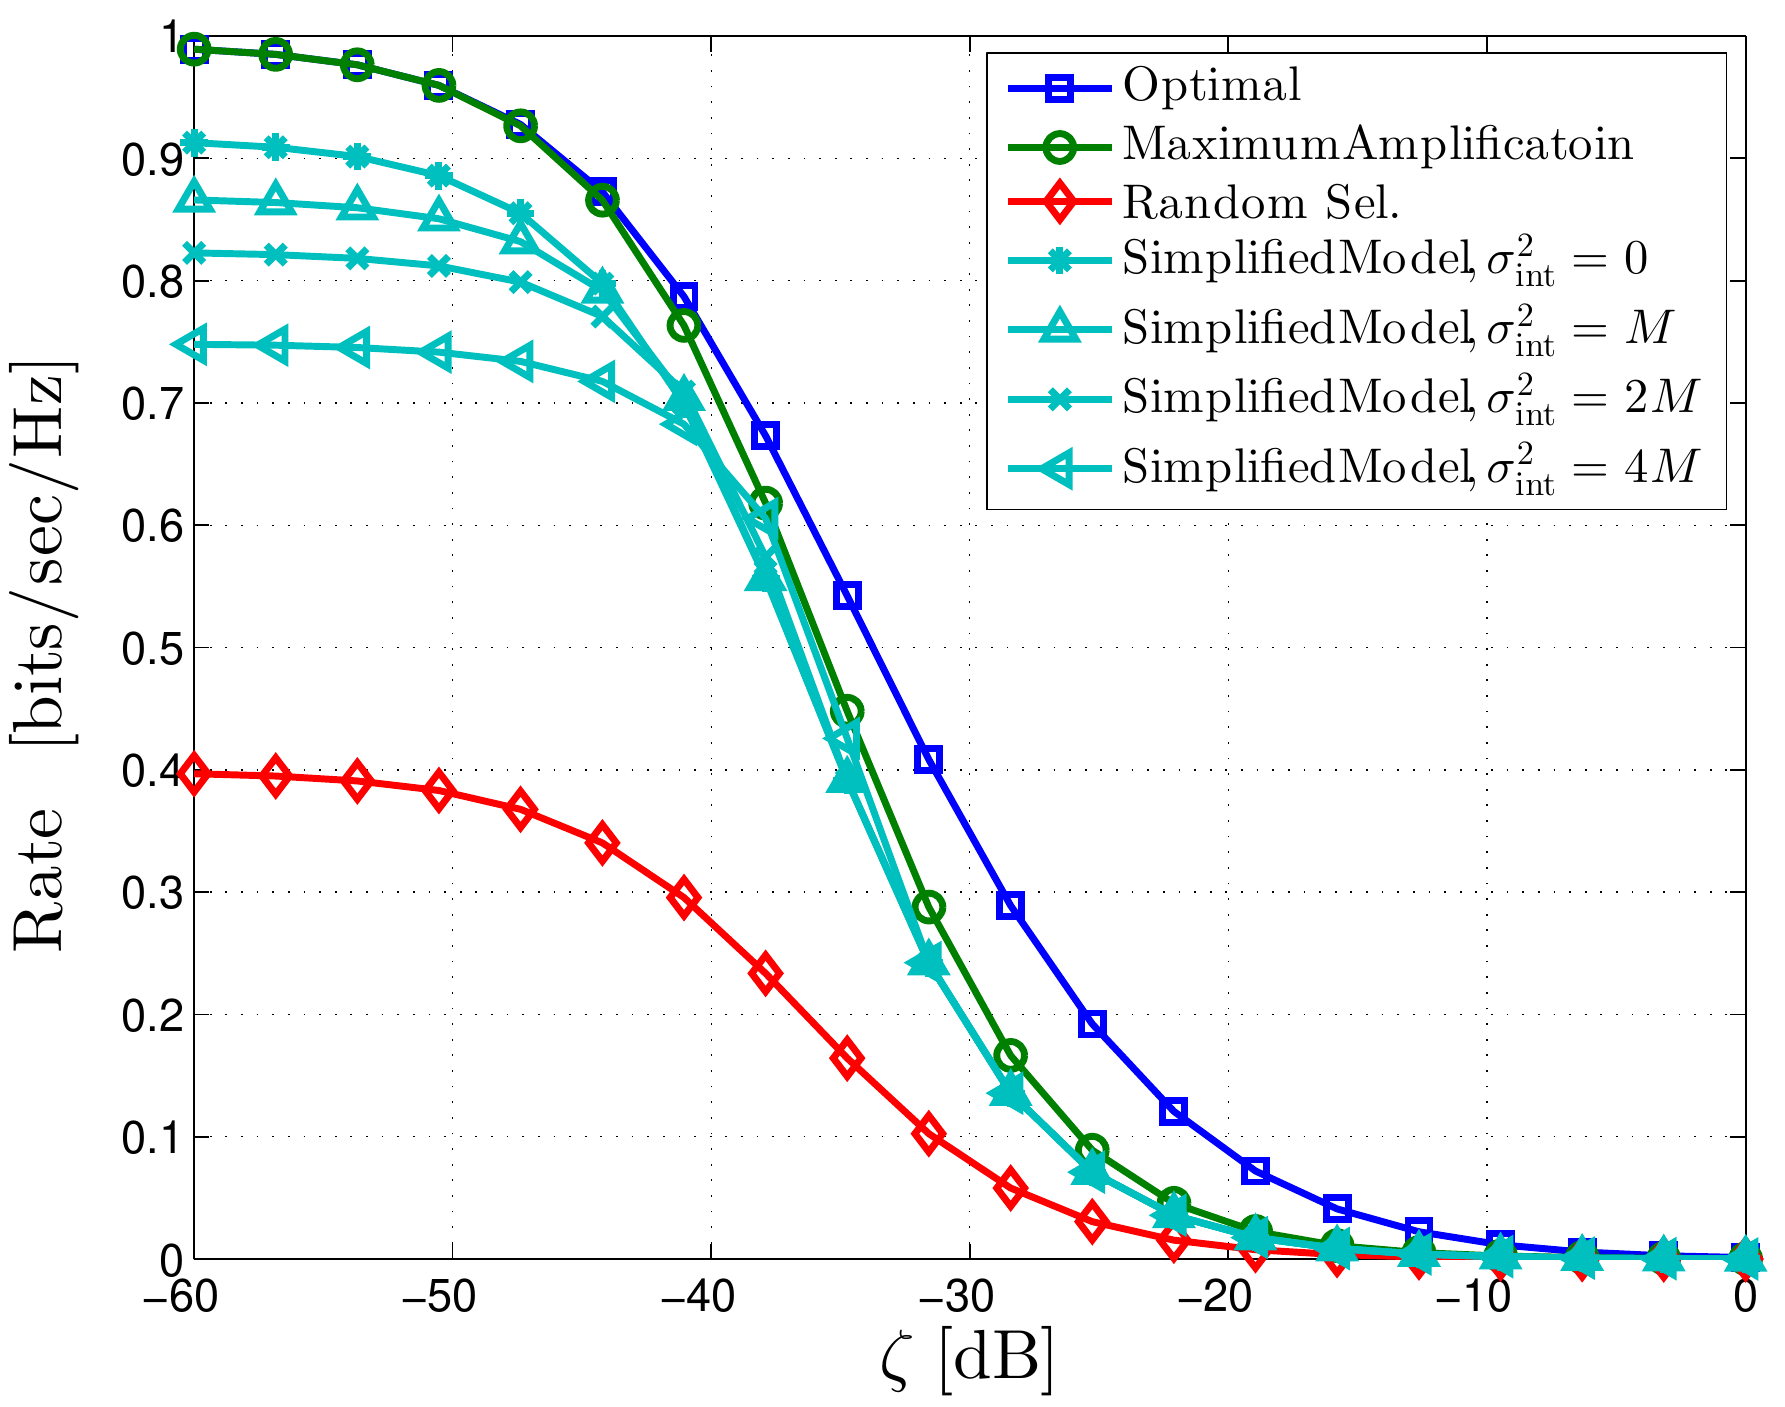}
				        %\fbox{model_rect6.pdf}
    \end{center} \vspace{-1mm}
    \caption{\small{Achievable rate [bits/sec/Hz] for the weakest end-to-end link vs. radius of the feasible channel estimation error set, i.e., $\mathcal{H}_k$, where $\zeta = \zeta_k, \forall k$. A relatively similar effect is observed compared to the distortion components, as they both result in higher residual interference at the relay. }}

\end{figure}
