# Supplementary material for: Hardware Impairments Aware Transceiver Design for Full-Duplex Amplify-and-Forward MIMO Relaying
Source: arXiv:1703.10209 source file (2017-08-15)
Supplement: Supplementary file 2 [file main_appendix_coefficients_calculate_alternating.tex]

Similar to the arguments in Appendix~\ref{appendix:coefficients}, the desired and error+noise power components, after the application of the reception filter, i.e., $\ma{z}$, is calculated as 
\begin{align} \label{eq:proof_appendix_p_des_afterZ} 
& \text{ derired received power at destination} \nonumber \\
& \;\;\;\;\;\;= P_{\text{s}} \ma{z}^H \ma{H}_{\text{rd}} {\ma{W}} \ma{h}_{\text{sr}}  \ma{h}_{\text{sr}}^H {\ma{W}}^H \ma{H}_{\text{rd}}^H \ma{z} \nonumber \\
& \;\;\;\;\;\;= {\omega}^2  P_{\text{s}} \left(\ma{z}^T \otimes \ma{z}^H \right) \left( \ma{H}_{\text{rd}}^* \otimes \ma{H}_{\text{rd}}  \right) \tilde{\ma{W}} \text{vec}\left( \ma{h}_{\text{sr}}  \ma{h}_{\text{sr}}^H \right) \nonumber \\
& \;\;\;\;\;\;= \bar{\omega} g_{\text{d}}, 
\end{align}
where $g_{\text{d}}$ is defined in (\ref{eq_ch_norm_coeffs_5}). Similarly, the noise+interference power can be calculated as  
\begin{align}
& \text{noise+interference power at destination} \nonumber \\
& \;\; = \sigma_{\text{nd}}^2 M_{\text{d}}   - g_{\text{d}}\bar{\omega}  + \ma{z}^H\ma{H}_{\text{rd}} \mathbb{E} \{ \ma{r}_{{\rm out}} \ma{r}_{{\rm out}}^{{H}} \} \ma{H}_{\text{rd}}^H \ma{z} \\
& \;\; = \sigma_{\text{nd}}^2 M_{\text{d}}   - a_{\text{d}}\bar{\omega}  + \left( \ma{z}^T \otimes \ma{z}^H \right) \left(\ma{H}_{\text{rd}}^{*} \otimes \ma{H}_{\text{rd}}  \right) \text{vec} \left(  \mathbb{E} \{ \ma{r}_{{\rm out}} \ma{r}_{{\rm out}}^{{H}} \} \right) \nonumber  \\
& \;\;=  \sigma_{\text{nd}}^2 M_{\text{d}}   - a_{\text{d}}\bar{\omega}  +  \left( \ma{z}^T \otimes \ma{z}^H \right) \left(\ma{H}_{\text{rd}}^{*} \otimes \ma{H}_{\text{rd}}  \right) \left( \ma{I}_{M_{\rm{r}}^2} + \gamma\ma{S}_{\text{D}} \right) \nonumber \\
& \quad\quad\quad\quad\quad\quad\quad\quad\quad \quad\quad \times \sum_{k\in\{0\cdots\infty\}} \left(\bar{\omega} \tilde{\ma{W}}  \ma{A} \right)^k \bar{\omega} \tilde{\ma{W}} \ma{a} \label{eq:appendix_coefficients_series_interference_excact_afterZ} \\
& \;\;\approx   \sum_{k\in\{1\cdots K \}}   \left( \ma{z}^T \otimes \ma{z}^H \right) \left(\ma{H}_{\text{rd}}^{*} \otimes \ma{H}_{\text{rd}}  \right) \left( \ma{I}_{M_{\rm{r}}^2} + \gamma\ma{S}_{\text{D}} \right) \nonumber \\
& \quad\quad\quad\quad\quad \quad\quad\quad\quad\quad\quad\times  \left(\tilde{\ma{W}}  \ma{A} \right)^{k-1}  \tilde{\ma{W}} \ma{a} \bar{\omega}^k \label{eq:appendix_coefficients_sqries_interference_approximation_afterZ} \\
& \;\;\approx \sum_{k\in\{0\cdots K \}} g_k \bar{\omega}^k,
\end{align} 
where $g_k$ is defined in (\ref{eq_ch_norm_coeffs_6}) and (\ref{eq_ch_norm_coeffs_7}). 
%Note that the identity in (\ref{eq:appendix_coefficients_series_interference_excact}) holds for any feasible relay transmit strategy, see (\ref{eq_loop_optimization_problem_b}). This stems from the fact that the effect of the distortion components are attenuated after passing through the loop process, i.e., $\tilde{\ma{W}}  \ma{A} $ in each consecutive symbol duration. Note that the contrary of this argument results in instability and infinite relay transmit power where the generated relay distortion is accumulated (and not attenuated) in subsequent symbol durations. It is worth mentioning that in a practical situation where the relay transmit power is well below infinity, the decreasing nature of the sequence presented by index $k$ is signified. Our numerical study shows that no significant performance gain is observed for $K>3$, considering the sub-optiomal nature of the proposed algorithm in Section~\ref{section:channel_norm_1}, see Algortihm~3.  
