# Supplementary material for: Hardware Impairments Aware Transceiver Design for Full-Duplex Amplify-and-Forward MIMO Relaying
Source: arXiv:1703.10209 source file (2017-08-15)
Supplement: Supplementary file 4 [file main_appendix_generalized_Rayl_Qotient.tex]

The optimization problem in (\ref{eq_ch_norm_W2_solution}) is equivalently written as 
\begin{align} \label{eq:GRQ_1}
\underset{\ma{W}_2}{\text{max}} \;\;\; & \frac{ \text{vec} \left( \ma{H}_{\text{rd}} \ma{W}_2 \right)^H  \text{vec} \left( \ma{H}_{2} \ma{W}_2 \right) } {\text{vec} \left( \ma{H}_{2} \ma{W}_2 \right)^H \text{vec} \left( \ma{H}_{2} \ma{W}_2 \right)  }, \;\; \text{s.t.} \;\;  \text{vec} \left(\ma{W}_2\right) = 1.  
\end{align}
Applying the matrix equalities \cite[e.q. (487), (486), (496)]{matrixcookbook}, (\ref{eq:GRQ_1}) is re-structured as 
\begin{align} \label{eq:GRQ_2}
\underset{\text{vec}(\ma{W}_2)}{\text{max}} \;\;\; & \frac{ \text{vec}(\ma{W}_2)^H \ma{C}_1 \text{vec}(\ma{W}_2) } { \text{vec}(\ma{W}_2)^H {\ma{C}}_2 \text{vec}(\ma{W}_2) }, \;\; \text{s.t.} \;\;  \text{vec} \left(\ma{W}_2\right) = 1,
\end{align}
where 
\begin{align} 
\ma{C}_1:= \ma{I}_{M_{\text{r}}} \otimes \left( \ma{H}_{\text{rd}}^H \ma{H}_{\text{rd}}\right),  \\
\ma{C}_2:= \ma{I}_{M_{\text{r}}} \otimes \left( \ma{H}_{2}^H \ma{H}_{2}\right), \label{eq:GRQ_2_C}
\end{align}
which is an explicit generalized Rayleigh quotient structure, with a known closed-form solution as $\lambda_{\text{max}} \left\{ \ma{C}_2^{-1}\ma{C}_1\}$, see \cite{GRQstructure}. The solution in (\ref{eq_ch_norm_W2_solution}) follows applying the matrix equality \cite[e.q. (488)]{matrixcookbook}. The solution in (\ref{eq_ch_norm_W1_solution}) is obtained following the similar steps as defined in (\ref{eq:GRQ_1})-(\ref{eq:GRQ_2_C}).
